# Supplementary material for: OmniEdit: Building Image Editing Generalist Models Through Specialist Supervision
Source: arXiv:2411.07199 source file (2025-04-28)
Supplement: Supplementary file 1 [file automatic_metric.tex]

\begin{tabular}{ccccccc}
                \toprule
                \textbf{Methods} & L1$\downarrow$ & L2$\downarrow$ & CLIP-I$\uparrow$ & CLIP-T$\uparrow$ & CLIP-Direct$\uparrow$ &  DINO$\uparrow$\\
                \midrule
                MagicBrush & 0.0646 & 0.022 & 0.8998 & 0.283 & 0.1388 & 0.8181 \\
                InstructPix2Pix & 0.1062 & 0.0296 & 0.8805 & 0.2942 & 0.1053 & 0.7954 \\
                UltraEdit & 0.0923 & 0.0237 & 0.825 & 0.309 & 0.1774 & 0.7082 \\
                DiffEdit & 0.043 & 0.0087 & 0.8775 & 0.2834 & 0.0873 & 0.8061 \\
                SDEdit & 0.1159 & 0.0296 & 0.8227 & 0.3289 & 0.1253 & 0.6876 \\
                CosXL-Edit & 0.0633 & 0.0166 & 0.9336 & 0.3154 & 0.1759 & 0.8816 \\
                HIVE & 0.114 & 0.0313 & 0.8177 & 0.2951 & 0.1479 & 0.681 \\
                HQ-Edit & 0.2215 & 0.0851 & 0.7282 & 0.2663 & 0.1018 & 0.5641 \\
                Omni-Edit & 0.066 & 0.0239 & 0.9035 & 0.3155 & 0.2004 & 0.7997 \\
                \bottomrule
\end{tabular}
